# Supplementary material for: Fundamental Limits of Low-Rank Matrix Estimation with Diverging Aspect Ratios
Source: arXiv:2211.00488 source file (2022-11-01)
Supplement: Supplementary file 1 [file appendix-lower-bound-part2.tex]

\section{Proof of Theorem \ref{thm:lower-bound}: upper bound}

In this section we assume support$(\Lambda) \subseteq [-K,K]$, support$(\Theta) \subseteq [-K,K]$, and $r = 1$. We will need to consider a model which is more general than \eqref{model:weak-signal}. In this model a small amount of side information is revealed, which allows us to prove the concentration of overlaps. Suppose we observe
\begin{align}
	& \bA = \frac{\sqrt{s}}{\sqrt[4]{nd}} \bLambda \bTheta^{\top} + \bZ, \label{model:general} \\
	& \bx = a'\sqrt{\ep_n'} \bLambda + \bg', \label{model:perturb-lambda} \\
	& \bx' = a\sqrt{\frac{n\ep_n}{d}} \bTheta + \bg\label{model:perturb-theta},  
\end{align}
where $\bg \sim \normal(0, \id_d)$, and $\bg' \sim \normal(0, \id_n)$ are independent of everything else. $a, a' \geq 0$, independent of $n,d$, $\epsilon_n, \epsilon_n' \rightarrow 0^+$ as $n,d \rightarrow 0$. We can associate to the observations in \eqref{model:general} the Hamiltonian 
\begin{align*}
	H_n^{(s)}(\vlambda, \vtheta) = \sum\limits_{i \in [n], j \in [d]}  \frac{s}{\sqrt{nd}} \Lambda_i \lambda_i \Theta_j \theta_j + \frac{\sqrt{s}}{\sqrt[4]{nd}} Z_{ij} \lambda_i \theta_j - \frac{s}{2\sqrt{nd}} \lambda_i^2 \theta_j^2.
\end{align*}
Note that $H_n^{(1)}(\vlambda, \vtheta) = H_n(\vlambda, \vtheta) $. Similarly, we can associate to the observations \eqref{model:perturb-lambda} and \eqref{model:perturb-theta} the following Hamiltonians:
\begin{align*}
	& \pertl(\vlambda) = \sum\limits_{i = 1}^n \sqrt{\ep_n'} a' \lambda_i g_i' + \ep_n'{a'}^2 \Lambda_i \lambda_i - \frac{{a'}^2 \ep_n}{2} \lambda_i^2, \\
	& \pertt(\vtheta) = \sum\limits_{j = 1}^d \sqrt{\frac{n\ep_n}{d}}a\theta_j g_j + \frac{n\ep_n}{d} a^2 \Theta_j \theta_j - \frac{a^2n\ep_n}{2d} \theta_j^2. 
\end{align*}
The ``total" Hamiltonian corresponding to all observations is defined as $\perttot(\vlambda, \vtheta) = H_n^{(s)}(\vlambda, \vtheta) + \pertl(\vlambda) + \pertt(\vtheta)$. Furthermore, we can define the corresponding free energy functional:
\begin{align*}
	& \Phi_n(s,a, a') = \frac{1}{n} \E\left[ \log \int \exp(\perttot(\vlambda, \vtheta) )\tensorl \tensort \right], \\
	& \phi_n(s, a, a') = \frac{1}{n}\log \int \exp(\perttot(\vlambda, \vtheta) )\tensorl \tensort. 
\end{align*}
Let $\Phi_n(a, a') = \Phi_n(1,a, a')$, $\phi_n( a, a') = \phi_n(1, a, a')$. We denote by $\langle \cdot\rangle_{n,s,a,a'}$ the posterior distribution given observations \eqref{model:general},\eqref{model:perturb-lambda} and \eqref{model:perturb-theta}, and let $\langle \cdot \rangle_{n,a,a'} = \langle \cdot\rangle_{n,1,a,a'}$ 
\begin{lemma}\label{lemma:G1}
	Assume $\|\Theta\|_{\infty}, \|\Lambda\|_{\infty} \leq K$, $d \gg n$, then for all $s > 0$, 
	\begin{align*}
		\lim\limits_{n,d \rightarrow \infty} \sup\limits_{a,a' \in [0,10]} \left| \Phi_n(s,a,a') - \sup\limits_{q \geq 0} \cF(\E[\Theta^2]^2s^2, q)\right| = 0.
	\end{align*} 
\end{lemma}
\begin{proof}
	Using Lemma \ref{lemma:free-energy-4} and Theorem 13 in \cite{lelarge2019fundamental}, we only need to prove 
	\begin{align*}
		\lim\limits_{n,d \rightarrow \infty}\sup\limits_{a,a' \in [0,10]} \left|\Phi_n(s,a,a') - \Phi_n(s,0,0) \right| = 0.
	\end{align*} 
	We prove this by taking derivative with respect to $\ep_n$ and $\ep_n'$,
	\begin{align*}
		\frac{\partial}{\partial \ep_n} \Phi_n(s,a,a') = \frac{a^2}{2d} \E[\langle \bTheta^{\top} \vtheta \rangle_{n,a}], \qquad \frac{\partial}{\partial \ep_n'} \Phi_n(s,a,a') = \frac{{a'}^2}{2n}\E[\langle \bLambda^{\top} \vlambda \rangle_{n,a}].
	\end{align*}
	Therefore $\sup\limits_{a,a' \in [0,10]} \left|\Phi_n(s,a,a') - \Phi_n(s,0,0) \right| \leq 50K^2(\ep_n + \ep_n') \rightarrow 0$ as $n,d \rightarrow \infty$, thus finishes the proof of this lemma. 
\end{proof}

Using Lemma \ref{lemma:convex-derivative}, Lemma \ref{lemma:free-energy-4}, Lemma \ref{lemma:G1} and Proposition 17 in \cite{lelarge2019fundamental}, we conclude that for Lebesgue almost everywhere $s\E[\Theta^2] > 0 $ and all $a,a' \in [0,10]$, if we take derivative of $\Phi_n(s,a,a')$ with respect to $s$ then apply Gaussian integration, we will get
\begin{align}\label{eq:G187}
	\lim\limits_{n,d \rightarrow \infty}\frac{1}{n\sqrt{nd}}\E\left[ \| \E[\bLambda \bTheta^{\top} \mid \bA, \bx, \bx'] - \E[\bLambda \bTheta^{\top} \mid \bA]  \|_F^2   \right] = 0. 
\end{align}
If we fix $s = 1$, then for Lebesgue almost everywhere $\E[\Theta^2] > 0 $ equation \eqref{eq:G187} still holds. In the rest part of the analysis, we will always assume $s = 1$. Notice that for all $a,a' \in [1,2]$, 
\begin{align*}
	\frac{1}{n\sqrt{nd}}\E\left[ \| \E[\bLambda \bTheta^{\top} \mid \bA, \bx, \bx'] - \E[\bLambda \bTheta^{\top} \mid \bA]  \|_F^2   \right] = & \frac{1}{n\sqrt{nd}}\E\left[ \| \langle \vlambda \vtheta^{\top}  \rangle_{n,a,a'} -  \langle \vlambda \vtheta^{\top}  \rangle_{n,0,0}  \|_F^2   \right] \\
	 \leq & \frac{1}{n\sqrt{nd}}\E\left[ \| \langle \vlambda \vtheta^{\top}  \rangle_{n,2,2} -  \langle \vlambda \vtheta^{\top}  \rangle_{n,0,0}  \|_F^2   \right], 
\end{align*}
thus
\begin{align*}
	\lim\limits_{n,d \rightarrow \infty}\int_1^2\int_1^2 \frac{1}{n\sqrt{nd}}\E\left[ \| \E[\bLambda \bTheta^{\top} \mid \bA, \bx, \bx'] - \E[\bLambda \bTheta^{\top} \mid \bA]  \|_F^2   \right] \dd a \dd a' = 0. 
\end{align*}
Then we take the following partial derivatives of the conditional entropy(differential entropy with respect to Lebesgue measure) and obtain
\begin{align*}
	& \frac{\partial }{\partial a'}H(\bLambda, \bTheta \mid \bA, \bx, \bx') = -\ep_n'a'\E\left[ \|\bLambda - \E[\bLambda \mid \bA, \bx, \bx']\|_F^2 \right], \\
	& \frac{\partial }{\partial a}H(\bLambda, \bTheta \mid \bA, \bx, \bx') = -\frac{\ep_n an}{d} \E\left[ \|\bTheta - \E[\bTheta \mid \bA, \bx, \bx']\|_F^2 \right], \\
	& \frac{\partial^2 }{\partial a \partial a'}H(\bLambda, \bTheta \mid \bA, \bx, \bx') = \frac{naa'\ep_n\ep_n'}{d}\E\left[ \|\E[\bLambda \bTheta^{\top} \mid \bA, \bx, \bx'] - \E[\bLambda \mid \bA, \bx, \bx'] \E[\bTheta^{\top} \mid \bA, \bx, \bx' ]\|_F^2  \right]. 
\end{align*}
Therefore, there exists $C>0$ depending only on $K$, such that
\begin{align*}
	 \int_1^2\int_1^2 \frac{1}{n\sqrt{nd}} \E\left[ \|\E[\bLambda^{\top} \bTheta \mid \bA, \bx, \bx'] - \E[\bLambda \mid \bA, \bx, \bx']\E[\bTheta^{\top} \mid \bA, \bx, \bx']\|_F^2 \right] \leq C d^{1/2}n^{-3/2} {\ep_n}^{-1}. 
\end{align*}
Combining \yw{scaling}

\begin{lemma}
	For $\vtheta \in \RR^d$, let 
	\begin{align*}
		U(\vtheta) = \sum\limits_{j = 1}^d \frac{1}{\sqrt{\ep_n nd}}\theta_j g_j + \frac{2a}{d} \theta_j \Theta_j - \frac{a}{d} \theta_j^2.
	\end{align*}
	Then under the conditions of Lemma \ref{lemma:G1}, for all $a \in [0,10]$,
	\begin{align*}
		\E\langle (\vtheta^{(1)} \cdot \vtheta^{(2)} - \E\langle \vtheta^{(1)} \cdot \vtheta^{(2)} \rangle_{n,a,a'})^2 \rangle_{n,a,a'} \leq 10K^2\E\langle | U(\vtheta) - \E\langle U(\vtheta) \rangle_{n,a,a'}|\rangle_{n,a,a'}. 
	\end{align*}
\end{lemma}
\begin{proof}
	
	Let $\vtheta^{(1)}$, $\vtheta^{(2)}$ be two independent samples from the posterior distribution $\langle \cdot \rangle_{n,a,a'}$. Since $\Theta$ has bounded support, we have
	\begin{align}
		\left| \E\langle U(\vtheta^{(1)}) \vtheta^{(1)}\cdot  \vtheta^{(2)} \rangle_{n,a,a'} - \E\langle \vtheta^{(1)} \cdot \vtheta^{(2)} \rangle_{n,a,a'} \E\langle U(\vtheta^{(1)}) \rangle_{n,a,a'}  \right| \leq K^2 \E\langle | U(\vtheta) - \E\langle U(\vtheta) \rangle_{n,a,a'}|\rangle_{n,a,a'}.\label{eq:G188}
	\end{align} 
	Using the property of Gaussian integration and Nishimori identity we have
	\begin{align}
		& \E\langle \vtheta^{(1)} \cdot \vtheta^{(2)} \rangle_{n,a,a'} \E\langle U(\vtheta^{(1)}) \rangle_{n,a,a'} = a\left( \E\langle \vtheta^{(1)} \cdot \vtheta^{(2)} \rangle_{n,a,a'} \right)^2,  \label{eq:G189}\\
		& \E\langle U(\vtheta^{(1)}) \vtheta^{(1)}\cdot  \vtheta^{(2)} \rangle_{n,a,a'} = a \E\langle (\vtheta^{(1)} \cdot \vtheta^{(2)})^2\rangle_{n,a,a'}. \label{eq:G190}  
	\end{align}
	Combining equations \eqref{eq:G188}, \eqref{eq:G189} and \eqref{eq:G190} we conclude that for all $a \in [0,10]$, 
	\begin{align*}
		\E\langle (\vtheta^{(1)} \cdot \vtheta^{(2)} - \E\langle \vtheta^{(1)} \cdot \vtheta^{(2)} \rangle_{n,a,a'})^2 \rangle_{n,a,a'} \leq 10K^2\E\langle | U(\vtheta) - \E\langle U(\vtheta) \rangle_{n,a,a'}|\rangle_{n,a,a'}. 
	\end{align*}
	 
\end{proof}

\begin{lemma}\label{lemma:G3}
	Let $v_n = \sup_{1/2 \leq a, a' \leq 3}\E[|\phi_n(a,a') - \E[\phi_n(a,a')]|] $. Under the conditions of Lemma \ref{lemma:G1}, 
	then there exists numerical constant $C_0 > 0$ depending only on $K$ such that
	\begin{align*}
		\int_1^2\int_1^2 \E\langle |U(\vtheta) - \E\langle U(\vtheta)\rangle_{n,a,a'}| \rangle_{n,a,a'}\dd a \dd a' \leq C_1 \sqrt{v_n\ep_n^{-1}}
	\end{align*}
\end{lemma}
\begin{proof}
	Notice that $\phi_n(a,a')$ is twice differentiable for $a,a' \in (0,10)$, and we can compute the partial derivatives:
	\begin{align}
		& \frac{\partial }{\partial a} \phi_n(a,a') = \ep_n \langle U(\vtheta) \rangle_{n,a,a'}, \nonumber \\
		& \frac{\partial^2 }{\partial a^2 } \phi_n(a,a') = n\ep_n^2\langle (U(\vtheta) - \langle U(\vtheta)\rangle_{n,a,a'})^2 \rangle_{n,a,a'} + \ep_n \langle 2\Theta\cdot \vtheta - \vtheta \cdot \vtheta \rangle_{n,a,a'}. \label{eq:G191}
	\end{align}
	Since $\Theta$ has bounded support, and $\left|\E[\frac{\partial }{\partial a} \phi_n(a,a')] \right| \leq  \ep_n a |\E\langle \bTheta \cdot \vtheta \rangle_{n,a,a'}| \leq 10 \ep_n K^2$ for $a \in (0,10)$, then we have
	\begin{align}
		& \langle (U(\vtheta) - \langle U(\vtheta)\rangle_{n,a,a'})^2 \rangle_{n,a,a'} \leq \frac{1}{n\ep_n^2}\left( \frac{\partial^2 }{\partial a^2 } \phi_n(a,a') + 3K^2\ep_n  \right), \nonumber\\
		& \int_1^2 \int_1^2 \E \langle (U(\vtheta) - \langle U(\vtheta)\rangle_{n,a,a'})^2 \rangle_{n,a,a'} \dd a \dd a' \nonumber \\
		 \leq & \int_1^2 \E\left[  \frac{1}{n\ep_n^2}\left( \frac{\partial }{\partial a} \phi_n(a,a')\Big\vert_{a = 2} - \frac{\partial }{\partial a} \phi_n(a,a')\Big\vert_{a = 1} + 3K^2\ep_n \right) \right] \dd a' \leq Cn^{-1}\ep_n^{-1}, \label{eq:G194}
	\end{align}
	where $C > 0$ is a numerical constant depending only on $K$. Furthermore, by equation \eqref{eq:191}, we can conclude that the following two functions are convex for all $a' \in (0,10)$:
	\begin{align*}
		 a \mapsto \phi_n(a,a') + \frac{3}{2}\ep_nK^2 a^2, \qquad a \mapsto \E[\phi_n(a,a')] + \frac{3}{2}\ep_nK^2 a^2. 
	\end{align*}
	Using Lemma \ref{lemma:convex-derivative}, we conclude that for all $a \in [1,2]$, $b \in (0, 1/2)$, we have
	\begin{align}
		\E \left[ \left| \frac{\partial }{\partial a} \phi_n(a,a') - E[ \frac{\partial }{\partial a} \phi_n(a,a')] \right| \right] \leq \E\left[ \frac{\partial }{\partial a} \phi_n(a + b,a') - \frac{\partial }{\partial a} \phi_n(a - b,a') \right] + 6\ep_nK^2b + \frac{3v_n}{b}. \label{eq:G192}
	\end{align}
	Again using the fact that $\left|\E[\frac{\partial }{\partial a} \phi_n(a,a')] \right| \leq  \ep_n a |\E\langle \bTheta \cdot \vtheta \rangle_{n,a,a'}| \leq 10 \ep_n K^2$ for $a \in (0,10)$, we have
	\begin{align}
		& \int_1^2 \E\left[ \frac{\partial }{\partial a} \phi_n(a + b,a') - \frac{\partial }{\partial a} \phi_n(a - b,a') \right] \dd a \nonumber \\
		 = & \E\left[ \phi_n(b + 2, a') - \phi_n(b + 1, a') - \phi_n(2 - b, a') + \phi_n(1 - b, a') \right] \leq C'K^2b\ep_n, \label{eq:G193}
	\end{align}
	where $C'$ is a numerical depending only on $K$. Combining equations \eqref{eq:G192} and \eqref{eq:G193} we get
	\begin{align*}
		\int_1^2\int_1^2 \E \left[ \left| \frac{\partial }{\partial a} \phi_n(a,a') - E[ \frac{\partial }{\partial a} \phi_n(a,a')] \right| \right] \dd a \dd a' \leq C''(b\ep_n + v_n / b),
	\end{align*}
	where $C''$ is a numerical constant depending only on $K$. Since $b$ can be any number in $(0,1/2)$, Lemma \ref{lemma:concentration-of-free-energy} shows that for $n,d$ large, $v_n < 1 / 4$, then we have
	\begin{align}\label{eq:G195}
		\int_1^2 \int_1^2 \E\left[ \left| \langle U(\vtheta)  \rangle_{n,a,a'} - \E \langle U(\vtheta)  \rangle_{n,a,a'} \right| \right] \dd a \dd a' \leq C'' \sqrt{v_n \ep_n^{-1}}. 
	\end{align} 
	Combining equations \eqref{eq:G194} and \eqref{G:195} finished the proof of this lemma. 
	
\end{proof}

\begin{lemma}\label{lemma:concentration-of-free-energy}
	Under the conditions of Lemma \ref{lemma:G1}, there exists numerical constant $C_1 > 0$ depending only on $K$, such that 
	\begin{align*}
		v_n \leq C_1 d^{1/2} n^{-1}. 
	\end{align*}
\end{lemma}
\begin{proof}
	Conditional on $(\bLambda, \bTheta)$, we consider the function 
	\begin{align*}
		f: (\bZ, \bg, \bg') \mapsto \phi_n(  a, a'). 
	\end{align*}
	It is not hard to see that for $n,d$ large enough, the following inequality holds for all $a,a' \in [0,10]$. 
	\begin{align*}
		\|\nabla f\|^2 \leq CK^4d^{1/2}n^{-3/2},
	\end{align*}
	where $C$ is a numerical constant. Applying Gaussian Poincar\'e inequality gives
	\begin{align}
	    \E_{\bZ, \bg, \bg'} \left[ \left( \phi_n(  a, a') - \E_{\bZ, \bg, \bg'}[\phi_n(  a, a')] \right)^2 \right] \leq CK^4d^{1/2}n^{-3/2}. \label{eq:conc187}
	\end{align}
	Then we show $\E_{\bZ, \bg, \bg'}[\phi_n( a, a')]$, which is a function of $(\bLambda, \bTheta)$, concentrates around its expectation. Notice that for $n,d$ large enough, for all $i \in [n], j \in [d]$ we have
	\begin{align*}
		& \left|\frac{\partial}{\partial \Lambda_i} \E_{\bZ, \bg, \bg'}[\phi_n( a, a')]\right| \leq C'K^3d^{1/2}n^{-3/2}, \\
		& \left|\frac{\partial}{\partial \Theta_j} \E_{\bZ, \bg, \bg'}[\phi_n(a, a')]\right| \leq C''K^3d^{-1/2}n^{-1/2},
	\end{align*} 
	where $C', C''$ are numerical constants. By Efron-Stein inequality, 
	\begin{align}
		\E\left[ \left(\E_{\bZ, \bg, \bg'}[\phi_n( a, a')] - \E[\phi_n(a, a')] \right)^2 \right] \leq C'''K^8dn^{-2}. \label{eq:conc188}
	\end{align}
	Combining \eqref{eq:conc187} and \eqref{eq:conc188} we conclude that for $n,d$ large enough, there exists a constant $C_1$ which depends only on $K$, such that for all $a,a' \in [0,10]$, 
	\begin{align*}
		\E\left[ \left(\phi_n( \ep_n, \ep_n', a, a') -  \E[\phi_n( \ep_n, \ep_n', a, a')] \right)^2 \right] \leq C_1^2 dn^{-2}, 
	\end{align*}
	thus the lemma follows by applying Cauchy–Schwarz inequality. 
\end{proof}

\begin{theorem}[Overlap concentration]
	Suppose $n^{6/5} \gg d \gg n$, $\Theta$, $\Lambda$ has bounded support, then we have
	\begin{align*}
		& \frac{d}{n}\int_1^2 \int_1^2 \E\langle (\vtheta^{(1)} \cdot \vtheta^{(2)} - \E\langle \vtheta^{(1)} \cdot \vtheta^{(2)} \rangle_{n,a,a'})^2  \rangle_{n,a,a'} \dd a \dd a' \rightarrow 0, \\
		& \int_1^2 \int_1^2 \E\langle (\vlambda^{(1)} \cdot \vlambda^{(2)} - \E\langle \vlambda^{(1)} \cdot \vlambda^{(2)} \rangle_{n,a,a'})^2  \rangle_{n,a,a'} \dd a \dd a' \rightarrow 0,
	\end{align*}
	as $n,d \rightarrow \infty$. 
\end{theorem}
