# Supplementary material for: Fundamental Limits of Low-Rank Matrix Estimation with Diverging Aspect Ratios
Source: arXiv:2211.00488 source file (2022-11-01)
Supplement: Supplementary file 2 [file appendix-lower-bound-part3.tex]

\section{Proof of Theorem \ref{thm:lower-bound}: lower bound}

In this section we assume support$(\Lambda) \subseteq [-K,K]$, support$(\Theta) \subseteq [-K,K]$, and $r = 1$. We will need to consider a model which is more general than \eqref{model:weak-signal}. In this model a small amount of side information is revealed. Specifically, suppose for $\ep_1, \ep_2 > 0 $, we observe
\begin{align}
	& \bA = \frac{1}{\sqrt[4]{nd}} \bLambda \bTheta^{\top} + \bZ, \label{model:general} \\
	& \bx(\ep_1) = \sqrt{\ep_1} \bLambda + \bg, \label{model:perturb-1} \\
	& \bY(\ep_2) = \frac{\sqrt{\ep_2}}{n} \bLambda \bLambda^{\top} + \bW. \label{model:perturb-2}
	%& \bx' = a\sqrt{\frac{n\ep_n}{d}} \bTheta + \bg\label{model:perturb-theta},  
\end{align}
where $\bg \sim \normal(0, \id_d)$, and $\bW \sim \frac{1}{\sqrt{d}} \GOE(n)$ are independent of everything else.  We can associate to the observations in \eqref{model:general} the Hamiltonian \eqref{eq:Hamiltonian}. Furthermore, we can associate to the observations \eqref{model:perturb-1} and \eqref{model:perturb-2} the following Hamiltonians:
\begin{align*}
	& \perta(\vlambda) = \sum\limits_{i = 1}^n \sqrt{\ep_1} \lambda_i g_i + \ep_1 \Lambda_i \lambda_i - \frac{ \ep_1}{2} \lambda_i^2, \\
	& \pertb(\vlambda) = \frac{\ep_2}{2n}\langle \bLambda, \vlambda \rangle^2 + \frac{\sqrt{\ep_2}}{2}\vlambda^\intercal\bW \vlambda - \frac{\ep_2}{4n}\|\vlambda\|_2^4. 
\end{align*}
The ``total" Hamiltonian corresponding to all observations is defined as $\perttot(\vlambda, \vtheta) = H_n(\vlambda, \vtheta) + \perta(\vlambda) + \pertb(\vlambda)$. Furthermore, we denote by $\langle \cdot\rangle_{n,\ep_1,\ep_2}$ the posterior distribution given observations \eqref{model:general},\eqref{model:perturb-1} and \eqref{model:perturb-2}, and we can define the corresponding free energy functional:
\begin{align*}
	& \Phi_n(\ep_1, \ep_2) = \frac{1}{n} \E\left[ \log \int \exp(\perttot(\vlambda, \vtheta) )\tensorl \tensort \right], \\
	& \phi_n(\ep_1, \ep_2) = \frac{1}{n}\log \int \exp(\perttot(\vlambda, \vtheta) )\tensorl \tensort. 
\end{align*}
Consider the conditional entropy $H(\bLambda, \bTheta \mid \bA, \bx(\ep_1), \bY(\ep_2))$, and take the following partial derivatives:
\begin{align*}
	& \frac{\partial }{\partial \ep_1}H(\bLambda, \bTheta \mid \bA, \bx(\ep_1), \bY(\ep_2)) = - \E\left[ \|\bLambda - \E[\bLambda \mid \bA, \bx(\ep_1), \bY(\ep_2)]\|^2 \right], \\
	%& \frac{\partial }{\partial a}H(\bLambda, \bTheta \mid \bA, \bx, \bx') = -\frac{\ep_n an}{d} \E\left[ \|\bTheta - \E[\bTheta \mid \bA, \bx, \bx']\|_F^2 \right], \\
	& \frac{\partial^2 }{\partial \ep_1^2}H(\bLambda, \bTheta \mid \bA, \bx(\ep_1), \bY(\ep_2)) = \E\left[ \|\E[\bLambda \bLambda^{\top} \mid \bA, \bx(\ep_1), \bY(\ep_2)] - \E[\bLambda \mid \bA, \bx(\ep_1), \bY(\ep_2)] \E[\bTheta^{\top} \mid \bA, \bx(\ep_1), \bY(\ep_2) ]\|_F^2  \right]. 
\end{align*}
Since $\|\bLambda\|_{\infty} \leq K$, then there exists numerical constant $C>0$ depending only on $K$, such that for any $\overline{\ep}_1 > \underline{\ep}_1 > 0$, 
\begin{align*}
	\frac{1}{n^2}\int_{\underline{\ep}_1}^{\overline{\ep}_1} \E\left[\|\E[\bLambda\bLambda^{\top} \mid \bA, \bx(\ep_1), \bY(\ep_2)] - \E[\bLambda \mid \bA, \bx(\ep_1), \bY(\ep_2) ]\E[\bLambda^{\top} \mid \bA, \bx(\ep_1), \bY(\ep_2) ]\|_F^2 \right] \dd \ep_1 \leq Cn^{-1}. 
\end{align*}
Let 
\begin{align*}
	E_n(\ep_1, \ep_2) = \frac{1}{n} \E\left[ \right]
\end{align*}
