# Supplementary material for: Fundamental Limits of Low-Rank Matrix Estimation with Diverging Aspect Ratios
Source: arXiv:2211.00488 source file (2022-11-01)
Supplement: Supplementary file 3 [file appendix-lower-bound-part4.tex]

\section{Proof of Theorem \ref{thm:lower-bound}: lower bound}

In this section we assume support$(\Lambda) \subseteq [-K,K]$, support$(\Theta) \subseteq [-K,K]$, and $r = 1$. We will need to consider a model which is more general than \eqref{model:weak-signal}. In this model a small amount of side information is revealed. Specifically, suppose $\ep, \ep' > 0$, and let $\bL \in \RR^n$ with the $i$-th coordinate being $L_i \iidsim \ber(\ep)$, $\bL' \in \RR^d$ with the $j$-th coordinate being $L_j' \iidsim \ber(\sqrt{n / d}\ep')$. Assume we have access to the following additional information apart from model \eqref{model:weak-signal}, for $i \in [n], j \in [d]$, let
\begin{align}\label{model:reveal}
	  x_i = \left\{ \begin{array}{ll}
		\Lambda_i & \mbox{if } L_i = 1, \\
		\ast & \mbox{if } L_i = 0. 
	\end{array} \right., \qquad x_j' = \left\{ \begin{array}{ll}
		\Theta_j & \mbox{if } L_j' = 1, \\
		\ast & \mbox{if } L_j' = 0. 
	\end{array} \right.,
\end{align}
where $x_i$ is the $i$-th coordinate of $\bx \in \RR^n$ and $x_j'$ is the $j$-th coordinate of $\bx' \in \RR^d$. $\ast$ is some value which does not belong to $\RR$. For $\vlambda \in \RR^n$, $\vtheta \in \RR^d$, we define the following notation
\begin{align*}
	& \barlambda = (\barlambda_1, \cdots, \barlambda_n) = (L_1\Lambda_1 + (1 - L_1)\lambda_1, \cdots, L_n\Lambda_n + (1 - L_n)\lambda_n), \\
	& \bartheta = (\bartheta_1, \cdots, \bartheta_d) = (L_1'\Theta_1 + (1 - L_1')\theta_1, \cdots, L_d'\Theta_d + (1 - L_d')\theta_d), \\
	& \tensorlb = \prod_{i \in [n], L_i = 0} \dd \mu_{\Lambda}(\lambda_i), \qquad \tensortb = \prod_{j \in [d], L_j' = 0} \dd \mu_{\Theta}(\theta_j), 
\end{align*} 
where $ \tensorlb $ is a probability distribution over $\RR^{n - \|\bL\|_1}$, and $\tensortb$ is a probability distribution over $\RR^{d - \|\bL'\|_1}$.  We can define the free energy associated to observations \eqref{model:weak-signal} and \eqref{model:reveal} as
\begin{align*}
	\Phi_{n, \ep, \ep'} = \frac{1}{n} \E\left[ \log \int \exp\left( H_n(\barlambda, \bartheta) \right) \tensorlb \tensortb \right].
\end{align*}
Recall that $H_n$ is as defined in \eqref{eq:Hamiltonian}. Then we show when $\ep, \ep'$ are small, $\Phi_{n,\ep, \ep'}$ and $\Phi_n$ are close. We follow a similar idea of Lemma \ref{lemma:free-energy-1}.

\begin{lemma}
	
\end{lemma}
\begin{proof}
Let $g(\cdot)$ be the density function for standard Gaussian distribution. For $k \in [d]$, let $\bar{P}_{\Theta,k}$ be a probability distribution over $\RR^{d - \|\bL'\|_1}$ defined as
$$\dd\bar{P}_{\Theta,k}(\vtheta) = \prod_{j \in [k], L_j' = 0}\dd\mu_{\Theta}(\theta_j) \prod_{j \in [d] \backslash [k], L_j' = 0} g(\theta_j)\dd \theta_j.$$
Furthermore, we define the following quantities:
	\begin{align*}
		\Phi_{n,\ep,\ep'}^{(k)} = \frac{1}{n} \E\left[ \log \int\exp(H_n(\barlambda, \bartheta)) \tensorlb \dd\bar{P}_{\Theta,k}(\vtheta)  \right].
	\end{align*}
	Furthermore, we define the following distributions over $\RR^{n + d - \|\bL\|_1 - \|\bL'\|_1}$
\end{proof}
