# Supplementary material for: Fundamental Limits of Low-Rank Matrix Estimation with Diverging Aspect Ratios
Source: arXiv:2211.00488 source file (2022-11-01)
Supplement: Supplementary file 4 [file appendix-lower-bound.tex]

\section{Proof of Theorem \ref{thm:lower-bound}}
\subsection{Computation of free energy} 
We first prove the result for $\Lambda$ having bounded support, and assume support$(\Lambda) \subseteq [-K,K]$. We also assume $\Theta$ is sub-gaussian with $\E[\Theta] = 0$, $\E[\Theta^3] = 0$, and $d / n \rightarrow \infty$. With a slight abuse of notations, in this section we will assume $A_{ij} = \frac{1}{\sqrt[4]{nd}} \Lambda_i \Theta_j + Z_{ij}$ with $\Lambda_i \iidsim \Lambda$ and $\Theta_j \iidsim \Theta$(integrated form being $\bA = \frac{1}{\sqrt[4]{nd}}\bLambda \bTheta^\intercal + \bZ$), and use the lower case letters $\lambda_i, \vlambda$, $\theta_j$ and $\vtheta$ as variables for posterior distributions. Define the Hamiltonian associated with the observations as:
\begin{align}\label{eq:Hamiltonian}
	H_n(\vlambda, \vtheta) = \frac{1}{\sqrt{nd}}\sum\limits_{i \in [n], j \in [d]} \Lambda_i\lambda_i \Theta_j \theta_j + \frac{1}{\sqrt[4]{nd}} \sum\limits_{i \in [n], j \in [d]} Z_{ij} \lambda_i \theta_j - \frac{1}{2\sqrt{nd}}\sum\limits_{i \in [n], j \in [d]}\lambda_i^2 \theta_j^2.
\end{align}
The posterior distribution of $\bLambda$ given $\bA$ is
\begin{align*}
	\mu_n(\vec{\lambda}) = \frac{1}{Z_n} \tensorl \int \exp\left(H_n(\vlambda, \vtheta)  \right)\tensort,
\end{align*}
with partition function
\begin{align*}
	Z_n = \int \exp\left(H_n(\vlambda, \vtheta)  \right)\tensort \tensorl.
\end{align*}
Then we show that the expected free energy density depends on $\Theta$ only through its second moment. 

\begin{lemma}\label{lemma:free-energy-1}
	Let $P_{\Theta, k}$ be a probability distribution over $\RR^d$ having independently distributed corrdinates, such that $\theta_1, \cdots, \theta_k \sim \Theta$, $\theta_{k + 1}, \cdots, \theta_d \sim \normal(0,q_{\Theta})$. Let $\Phi_n^{(k)}$ be the expected free energy density corresponding to $P_{\Theta, k}$: 
	\begin{align*}
		\Phi_n^{(k)} = \frac{1}{n} \E\left[ \log \left( \int \exp(H_n(\vlambda, \vtheta)) \tensorl \dd P_{\Theta, k}(\vtheta) \right) \right].
	\end{align*}	
	Let $\Phi_n = \Phi_n^{(d)}$. Then under assumptions $\E[\Theta] = \E[\Theta^3] = 0$, $\Theta$ is sub-gaussian, support$(\Lambda) \subseteq[-K,K]$ and $d / n \rightarrow \infty$,  $\Phi_n^{(d)} - \Phi_n^{(0)} = o(1)$. 
\end{lemma}

\begin{proof}
	For $k \in [d]$, let
	\begin{align*}
		H_n^{(k)}(\vlambda, \vtheta) = \frac{1}{\sqrt{nd}}\sum\limits_{i = 1}^n \sum\limits_{j = 1, j \neq k}^d \Lambda_i\lambda_i \Theta_j \theta_j + \frac{1}{\sqrt[4]{nd}}\sum\limits_{i = 1}^n \sum\limits_{j = 1, j \neq k}^d Z_{ij} \lambda_i \theta_j- \frac{1}{2\sqrt{nd}}\sum\limits_{i = 1}^n \sum\limits_{j = 1, j \neq k}^d \lambda_i^2 \theta_j^2. 
	\end{align*}
	Furthermore, for $k \in [d]$, define the following distributions as well as the corresponding partition functions:
	\begin{align*}
		& \mu_n^{(k,+)}(\vlambda, \vtheta) = \frac{1}{Z_n^{(k,+)}} \exp\left( H_n^{(k)}(\vlambda, \vtheta) \right) \tensorl \dd P_{\Theta, k}(\vtheta), \\
		& Z_n^{(k, +)} = \int \exp\left( H_n^{(k)}(\vlambda, \vtheta) \right) \tensorl \dd P_{\Theta, k}(\vtheta), \\
		& \mu_n^{(k,-)}(\vlambda, \vtheta) = \frac{1}{Z_n^{(k,-)}} \exp\left( H_n^{(k)}(\vlambda, \vtheta) \right) \tensorl \dd P_{\Theta, k - 1}(\vtheta), \\
		& Z_n^{(k, -)} = \int \exp\left( H_n^{(k)}(\vlambda, \vtheta) \right) \tensorl \dd P_{\Theta, k - 1}(\vtheta).
	\end{align*}
	Note that despite introducing various ``posterior-like" distributions, the distribution of the data remains unchanged as proposed in model \eqref{model:weak-signal}. Since $H_n^{(k)}(\vlambda, \vtheta)$ is by definition independent of $\theta_k$, for every observation we have $Z_n^{(k, +)} = Z_n^{(k, -)}$, and further
	\begin{align*}
		& \Phi_n^{(k)} - \Phi_n^{(k - 1)} =\frac{1}{n} \E\left[ \log \left( \mu_n^{(k, +)}\left[\exp(h_n^{(k)}(\vlambda, \vtheta)  )\right) \right] \right] - \frac{1}{n}\E\left[ \log \left( \mu_n^{(k, -)}\left[\exp(h_n^{(k)}(\vlambda, \vtheta)  )\right) \right] \right],
	\end{align*}
	where $h_n^{(k)}(\vlambda, \vtheta) = H_n(\vlambda, \vtheta) - H_n^{(k)}(\vlambda, \vtheta)$, and $ \mu_n^{(k, +)}[X]$, $ \mu_n^{(k, -)}[X]$ are the expectations of random variable $X$ under distributions $\mu_n^{(k, +)}, \mu_n^{(k, -)}$, respectively. Further, let $\bZ_{\cdot k} \in \RR^n$ be the $k$-th column of matrix $\bZ$. 
	
For $k \in [d]$, consider the Taylor expansion
\begin{align*}
	\exp\left(h_n^{(k)}(\vlambda, \vtheta) \right) = 1 + \sum\limits_{l = 1}^4 c_l^{(k)} \theta_k^l + R^{(k)} + \sum\limits_{l = 5}^{\infty} \frac{1}{l!}h_n^{(k)}(\vlambda, \vtheta)^l,
\end{align*}
where
\begin{align*}
	 c_1^{(k)} =& \frac{1}{\sqrt{nd}} \langle \bLambda, \vlambda \rangle \Theta_k + \frac{1}{\sqrt[4]{nd}} \langle \bZ_{\cdot k}, \vlambda \rangle, \\
	 c_2^{(k)} =& \frac{1}{2}\left( \frac{1}{\sqrt{nd}} \langle \bLambda, \vlambda \rangle \Theta_k + \frac{1}{\sqrt[4]{nd}} \langle \bZ_{\cdot k}, \vlambda\rangle \right)^2 - \frac{1}{2\sqrt{nd}} \langle \vlambda, \vlambda \rangle, \\
	 c_3^{(k)} =& -\frac{1}{2nd}  \langle \bLambda, \vlambda \rangle  \langle \vlambda, \vlambda \rangle \Theta_k  - \frac{1}{2n^{3/4}d^{3/4}}  \langle  \bZ_{\cdot k} , \vlambda \rangle \langle  \vlambda, \vlambda \rangle  + \frac{1}{6} \left( \frac{1}{\sqrt{nd}} \langle \bLambda, \vlambda \rangle \Theta_k + \frac{1}{\sqrt[4]{nd}} \langle \bZ_{\cdot k}, \vlambda \rangle \right)^3, \\
	c_4^{(k)} = & \frac{1}{8nd}\langle \vlambda, \vlambda \rangle^2 - \frac{1}{4\sqrt{nd}} \langle \vlambda, \vlambda \rangle\left( \frac{1}{\sqrt{nd}} \langle \bLambda, \vlambda \rangle \Theta_k + \frac{1}{\sqrt[4]{nd}} \langle \bZ_{\cdot k}, \vlambda  \rangle \right)^2 + \frac{1}{24}\left(\frac{1}{\sqrt{nd}} \langle \bLambda, \vlambda \rangle \Theta_k + \frac{1}{\sqrt[4]{nd}} \langle \bZ_{\cdot k}, \vlambda \rangle \right)^4, \\
	R^{(k)}  = & - \frac{\langle \vlambda, \vlambda \rangle^3}{48(nd)^{3/2}}  \theta_k^6 + \frac{1}{24nd} \langle \vlambda, \vlambda \rangle^2 \left(\frac{1}{\sqrt{nd}} \langle \bLambda, \vlambda \rangle \Theta_k + \frac{1}{\sqrt[4]{nd}} \langle \bZ_{\cdot k}, \vlambda \rangle \right) \theta_k^5 + \frac{1}{384n^2d^2} \langle \vlambda, \vlambda \rangle^4 \theta_k^8\\
	&  - \frac{1}{12\sqrt{nd}} \langle \vlambda, \vlambda \rangle   \left( \frac{1}{\sqrt{nd}} \langle \bLambda, \vlambda \rangle \Theta_k + \frac{1}{\sqrt[4]{nd}} \langle \bZ_{\cdot k}, \vlambda \rangle \right)^3 \theta_k^5 + \frac{1}{16nd} \langle \vlambda, \vlambda \rangle^2 \left( \frac{1}{\sqrt{nd}} \langle \bLambda, \vlambda \rangle \Theta_k + \frac{1}{\sqrt[4]{nd}} \langle \bZ_{\cdot k}, \vlambda \rangle \right)^2 \theta_k^6\\
	&   -\frac{1}{48(nd)^{3/2}}  \langle \vlambda, \vlambda \rangle^3 \left( \frac{1}{\sqrt{nd}} \langle \bLambda, \vlambda \rangle \Theta_k + \frac{1}{\sqrt[4]{nd}} \langle \bZ_{\cdot k} , \vlambda \rangle \right) \theta_k^7.
\end{align*}
Under distribution $\mu_n^{(k, +)}$, $\theta_k \sim \Theta$, and is independent of $(\vtheta_{-k}, \vlambda)$. By assumption $\E[\Theta] = \E[\Theta^3] = 0$, thus we have
\begin{align*}
	\mu_n^{(k, +)}\left[ \exp\left(h_n^{(k)}(\vlambda, \vtheta) \right) \right] = 1 + \mu_n^{(k, +)}[c_2^{(k)}]q_{\Theta} + \mu_n^{(k, +)}[c_4^{(k)}]\E[\Theta^4] + \sum\limits_{l = 5}^{\infty} \frac{1}{l!}\mu_n^{(k, +)}[h_n^{(k)}(\vlambda, \vtheta)^l].
\end{align*}
Notice that $c_2^{(k)} \geq -\frac{1}{2} \sqrt{\frac{n}{d}}K^2$, 
\begin{align*}
	 \frac{3}{8nd} \langle \vlambda, \vlambda \rangle^2- \frac{1}{4\sqrt{nd}}\langle \vlambda, \vlambda \rangle \left( \frac{1}{\sqrt{nd}} \langle \bLambda, \vlambda  \rangle \Theta_k + \frac{1}{\sqrt[4]{nd}} \langle \bZ_{\cdot k}, \vlambda \rangle \right)^2 +\frac{1}{24}\left(\frac{1}{\sqrt{nd}} \langle \bLambda, \vlambda \rangle \Theta_k + \frac{1}{\sqrt[4]{nd}} \langle \bZ_{k \cdot}, \vlambda \rangle \right)^4 \geq 0,
\end{align*}
thus $c_4^{(k)} \geq -\frac{1}{4nd} \langle \vlambda, \vlambda \rangle^2 \geq -\frac{n}{4d} K^4$. Furthermore, by Jensen's inequality,  
\begin{align*}
	\mu_n^{(k, +)}\left[ \exp\left(h_n^{(k)}(\vlambda, \vtheta) \right) \right] \geq \exp\left( \mu_n^{(k, +)}\left[ h_n^{(k)}(\vlambda, \vtheta) \right] \right) \geq \exp\left( - \frac{1}{2}\sqrt{\frac{n}{d}}K^2 q_{\Theta} \right),
\end{align*}
thus by the concavity of $\log(1 + x)$ we have
\begin{align}
	& \left|\log\left( \mu_n^{(k, +)}\left[ \exp\left(h_n^{(k)}(\vlambda, \vtheta) \right) \right] \right) - \log\left( 1 + \mu_n^{(k, +)}[c_2^{(k)}]q_{\Theta} + \mu_n^{(k, +)}[c_4^{(k)}]\E[\Theta^4] \right)\right| \nonumber\\
	\leq & \left|\sum\limits_{l = 5}^{\infty} \frac{1}{l!}\mu_n^{(k, +)}[h_n^{(k)}(\vlambda, \vtheta)^l] \right| \times \max\left\{ {\mu_n^{(k, +)}\left[ \exp\left(h_n^{(k)}(\vlambda, \vtheta) \right) \right]}^{-1}, \left( 1 + \mu_n^{(k, +)}[c_2^{(k)}]q_{\Theta} + \mu_n^{(k, +)}[c_4^{(k)}]\E[\Theta^4] \right)^{-1} \right\} \nonumber \\
	\leq & \left|\sum\limits_{l = 5}^{\infty} \frac{1}{l!}\mu_n^{(k, +)}[h_n^{(k)}(\vlambda, \vtheta)^l] \right| \times \max\left\{ \exp\left(  \frac{1}{2}\sqrt{\frac{n}{d}}K^2 q_{\Theta} \right), \left( 1  -\frac{1}{2} \sqrt{\frac{n}{d}}K^2q_{\Theta} -\frac{n}{4d}K^4\E[\Theta^4] \right)^{-1}    \right\}. 
\end{align}
By sub-gaussian properties, there exists numerical constant $C > 0$, such that for any $p \in \NN^+$, $\E[|\Theta|^p] \leq C^p p^{p/2}$, $\E[|G|^p] \leq C^p p^{p/2}$ with $G \sim \normal(0,1)$. Note that in the following equations, $\E[\cdot]$ stands for taking expectation over the randomness of data matrix $\bA$, then we have
\begin{align*}
	& \E \left[ \left|\sum\limits_{l = 5}^{\infty} \frac{1}{l!}\mu_n^{(k, +)}[h_n^{(k)}(\vlambda, \vtheta)^l] \right|  \right] \\
	\leq & \sum\limits_{l = 5}^{\infty} \frac{1}{l!} \E\left[ \mu_n^{(k, +)}\left[ \left|  \frac{1}{\sqrt{nd}} \langle \bLambda, \vlambda \rangle \Theta_k \theta_k + \frac{1}{\sqrt[4]{nd}}\langle \bZ_{\cdot k}, \vlambda \rangle \theta_k - \frac{1}{2\sqrt{nd}}\langle \vlambda, \vlambda \rangle \theta_k^2 \right|^l \right]   \right] \\
	\leq & \sum\limits_{l = 5}^{\infty} \frac{1}{l!}\E\left[ \mu_n^{(k, +)}\left[ \left|  \frac{1}{\sqrt{nd}} \langle \bLambda, \vlambda \rangle \Theta_k \theta_k + \frac{1}{\sqrt[4]{nd}} \langle \bZ_{\cdot k}, \vlambda \rangle \theta_k - \frac{1}{2\sqrt{nd}}\langle \vlambda, \vlambda \rangle \theta_k^2 \right|^{2l}\right]   \right]^{1/2} \\
	\leq & \sum\limits_{l = 5}^{\infty} \frac{3^l}{l!}\times \left\{ \E\left[\mu_n^{(k, +)}\left[\left| \frac{1}{\sqrt{nd}} \langle \bLambda, \vlambda \rangle\Theta_k \theta_k \right|^{2l} \right] \right]^{1/2} + \E\left[\mu_n^{(k, +)}\left[\left| \frac{1}{\sqrt[4]{nd}} \langle \bZ_{\cdot k}, \vlambda_i \rangle \theta_k \right|^{2l} \right] \right]^{1/2} + \right.\\
	& \left. \E\left[\mu_n^{(k, +)}\left[\left| \frac{1}{2\sqrt{nd}}\langle \vlambda, \vlambda \rangle \theta_k^2 \right|^{2l} \right] \right]^{1/2}  \right\} \\
	\leq & \sum\limits_{l = 5}^{\infty} \frac{3^l}{l!}\times \left\{\frac{K^{2l}C^{2l}n^{l/2}}{d^{l/2}} \times (2l)^l + \frac{K^lC^{2l}n^{l/4}}{d^{l/4}} \times (2l)^l + \frac{K^{2l}C^{2l}n^{l/2}}{d^{l/2}}\times (2l)^l \right\}  \lesssim  \frac{n^{5/4}}{d^{5/4}}.
\end{align*}
Summing over $k$ gives
\begin{align}\label{eq:219}
	\left|\sum\limits_{k = 1}^d \frac{1}{n} \E\left[ \log\left( \mu_n^{(k, +)}\left[ \exp\left(h_n^{(k)}(\vlambda, \vtheta) \right) \right] \right) - \log\left( 1 + \mu_n^{(k, +)}[c_2^{(k)}]q_{\Theta} + \mu_n^{(k, +)}[c_4^{(k)}]\E[\Theta^4] \right) \right]\right| \lesssim \frac{n^{1/4}}{d^{1/4}} = o(1).
\end{align}
Again applying concavity of $\log(x + 1)$, we have
\begin{align}
	&  \log\left( 1 + \mu_n^{(k, +)}[c_2^{(k)}] q_{\Theta} \right) +  \mu_n^{(k, +)}[c_4^{(k)}]\E[\Theta^4] - \frac{|\mu_n^{(k, +)}[c_4^{(k)}]\E[\Theta^4]\left(\mu_n^{(k, +)}[c_2^{(k)}] q_{\Theta} + \mu_n^{(k, +)}[c_4^{(k)}] \E[\Theta^4]\right)|}{1 + \mu_n^{(k, +)}[c_2^{(k)}] q_{\Theta} + \mu_n^{(k, +)}[c_4^{(k)}] \E[\Theta^4]} \nonumber \\
	\leq & \log\left( 1 + \mu_n^{(k, +)}[c_2^{(k)}] q_{\Theta} \right) + \frac{\mu_n^{(k, +)}[c_4^{(k)}]\E[\Theta^4]}{1 + \mu_n^{(k, +)}[c_2^{(k)}] q_{\Theta} + \mu_n^{(k, +)}[c_4^{(k)}] \E[\Theta^4]} \nonumber\\
	\leq & \log \left(1 + \mu_n^{(k, +)}[c_2^{(k)}]q_{\Theta} + \mu_n^{(k, +)}[c_4^{(k)}] \E[\Theta^4] \right) \leq \log\left( 1 + \mu_n^{(k, +)}[c_2^{(k)}] q_{\Theta} \right) + \frac{\mu_n^{(k, +)}[c_4^{(k)}]\E[\Theta^4]}{1 + \mu_n^{(k, +)}[c_2^{(k)}]q_{\Theta} }\nonumber \\
	 \leq & \log\left( 1 + \mu_n^{(k, +)}[c_2^{(k)}] q_{\Theta} \right) +  \mu_n^{(k, +)}[c_4^{(k)}]\E[\Theta^4] + \frac{|\mu_n^{(k, +)}[c_2^{(k)}]\mu_n^{(k, +)}[c_4^{(k)}]q_{\Theta}\E[\Theta^4]|}{1 + \mu_n^{(k, +)}[c_2^{(k)}]q_{\Theta}}. \label{eq:220}
\end{align}
Notice that under the composite distribution $P_{\bA}(\bLambda, \bTheta, \bZ) \otimes \mu_n^{(k, +)}(\vlambda, \vtheta)$, $\{Z_{ik}: i \in [n]\}$, $\Theta_k$, $\{\lambda_i, \Lambda_i: i \in [n]\}$, and $\theta_k$ are independent of each other. Then we have
\begin{align*}
	\E\left[\mu_n^{(k, +)}\left[ \frac{1}{8nd} \langle \vlambda, \vlambda \rangle^2 - \frac{1}{4nd} \langle \vlambda, \vlambda \rangle \langle\bZ_{\cdot k}, \vlambda \rangle^2 + \frac{1}{24nd}\langle \bZ_{\cdot k}, \vlambda \rangle^4  \right]  \right] = 0,
\end{align*}
thus deducing from the expression of $c_4^{(k)}$
\begin{align}\label{eq:221}
	\left| \E[\mu_n^{(k, +)}[c_4^{(k)}]]  \right| \leq \frac{n^{3/2}}{2d^{3/2}}K^6q_{\Theta} + \frac{n^2}{24d^2}K^8 \E[\Theta^4].
\end{align}
Further, notice that 
\begin{align}
	& \E\left[\frac{|\mu_n^{(k, +)}[c_2^{(k)}]\mu_n^{(k, +)}[c_4^{(k)}]q_{\Theta}\E[\Theta^4]|}{1 + \mu_n^{(k, +)}[c_2^{(k)}]q_{\Theta}} \right] \lesssim \frac{1}{1-\frac{1}{2} \sqrt{\frac{n}{d}}K^2q_{\Theta}} \times \frac{n^{3/2}}{d^{3/2}}, \label{eq:222}\\
	& \E\left[ \frac{|\mu_n^{(k, +)}[c_4^{(k)}]\E[\Theta^4]\left(\mu_n^{(k, +)}[c_2^{(k)}] q_{\Theta} + \mu_n^{(k, +)}[c_4^{(k)}] \E[\Theta^4]\right)|}{1 + \mu_n^{(k, +)}[c_2^{(k)}] q_{\Theta} + \mu_n^{(k, +)}[c_4^{(k)}] \E[\Theta^4]} \right] \lesssim \frac{1}{1 -\frac{1}{2} \sqrt{\frac{n}{d}}K^2q_{\Theta} -\frac{n}{4d} K^4 \E[\Theta^4]} \times \frac{n^{3/2}}{d^{3/2}}.  \label{eq:223}
\end{align}
Take expectation over the inequalities in \eqref{eq:220}, and apply \eqref{eq:221}, \eqref{eq:222}, \eqref{eq:223}, then sum over $k$, we get 
\begin{align*}
	& \sum\limits_{k = 1}^d \frac{1}{n} \E\left[\log\left( 1 + \mu_n^{(k, +)}[c_2^{(k)}] q_{\Theta} \right) \right] - \frac{Cn^{1/2}}{d^{1/2}} \\
	\leq & \sum\limits_{k = 1}^d \frac{1}{n} \E\left[ \log \left(1 + \mu_n^{(k, +)}[c_2^{(k)}]q_{\Theta} + \mu_n^{(k, +)}[c_4^{(k)}] \E[\Theta^4] \right) \right] \\
	 \leq & \sum\limits_{k = 1}^d \frac{1}{n} \E\left[\log\left( 1 + \mu_n^{(k, +)}[c_2^{(k)}] q_{\Theta} \right) \right] + \frac{Cn^{1/2}}{d^{1/2}},
\end{align*}
where $C$ is a numerical constant. Taking $n,d \rightarrow \infty$, and combine the above equations with \eqref{eq:219} we have
\begin{align*}
	\sum\limits_{k = 1}^d \frac{1}{n} \E\left[\log\left( 1 + \mu_n^{(k, +)}[c_2^{(k)}] q_{\Theta} \right) \right] - \sum\limits_{k = 1}^d \frac{1}{n} \E\left[ \log\left( \mu_n^{(k, +)}\left[ \exp\left(h_n^{(k)}(\vlambda, \vtheta) \right) \right] \right)\right] = o(1).
\end{align*}
Similarly, we can show
\begin{align*}
	\sum\limits_{k = 1}^d \frac{1}{n} \E\left[\log\left( 1 + \mu_n^{(k, -)}[c_2^{(k)}] q_{\Theta} \right) \right] - \sum\limits_{k = 1}^d \frac{1}{n} \E\left[ \log\left( \mu_n^{(k, -)}\left[ \exp\left(h_n^{(k)}(\vlambda, \vtheta) \right) \right] \right)\right] = o(1).
\end{align*}
Since $c_2^{(k)}$ is independent of $\theta_k$, for all $(\bLambda, \bTheta, \bZ)$ we have $\mu_n^{(k, +)}[c_2^{(k)}] = \mu_n^{(k,-)}[c_2^{(k)}]$, thus $\Phi_n^{(d)}- \Phi_n^{(0)} = o(1)$, completing the proof of this lemma. 

\end{proof}

Notice that it is convenient to compute $\Phi_n^{(0)}$ by Gaussian integration. By computing its value we find that $\Phi_n^{(0)}$ can be well approximated by a quantity stated in the following lemma:
\begin{lemma}\label{lemma:free-energy-2}
Let 
\begin{align*}
	\tilde{\Phi}_n = { \frac{1}{n} \E\left[ \log \left( \int \exp\left(\frac{q_{\Theta}^2}{2n}\langle \bLambda, \vlambda \rangle^2 + \frac{q_{\Theta}\left\| \frac{1}{\sqrt[4]{nd}} \bZ^\intercal \vlambda \right\|_2^2}{2} - \frac{dq_{\Theta}}{2\sqrt{nd}}\|\vlambda\|_2^2 - \frac{q_{\Theta}^2}{4n}\|\vlambda\|_2^4 \right) \tensorl \right) \right]}.
\end{align*}
Under the assumptions stated in Lemma \ref{lemma:free-energy-1}, we have $\tilde{\Phi}_n - \Phi_n^{(0)} = o(1)$. 
\end{lemma}
\begin{proof}
	By Gaussian integration, we have
	\begin{align*}
	 \Phi_n^{(0)} =& \frac{1}{n} \E\left[ \log \left( \int \exp \left( \frac{ \frac{1}{{nd}}\langle \bLambda, \vlambda \rangle^2 \|\bTheta\|_2^2}{2q_{\Theta}^{-1} + \frac{2}{\sqrt{nd}}\|\vlambda\|_2^2} + \frac{\frac{1}{(nd)^{3/4}}\langle \bLambda, \vlambda \rangle \langle \vlambda ,\bZ\bTheta \rangle}{q_{\Theta}^{-1} + \frac{1}{\sqrt{nd}}\|\vlambda\|_2^2} + \right.\right.\right.\\
	&\left.\left.\left. \frac{\left\| \frac{1}{\sqrt[4]{nd}} \bZ^\intercal \vlambda \right\|_2^2}{2q_{\Theta}^{-1} + \frac{2}{\sqrt{nd}} \|\vlambda\|_2^2} - \frac{d}{2}\log\left( 1 + \frac{q_{\Theta}}{\sqrt{nd}}\|\vlambda\|_2^2 \right) \right) \tensorl\right) \right].
\end{align*}
Then we analyze the above equation part by part, and obtain the following inequalities:
\begin{align}
	& \sup\limits_{\|\vlambda\|_{\infty} \leq K} \left| \frac{ \frac{1}{{nd}}\langle \bLambda, \vlambda \rangle^2 \|\bTheta\|_2^2}{2q_{\Theta}^{-1} + \frac{2}{\sqrt{nd}}\|\vlambda\|_2^2} - \frac{q_{\Theta}^2}{2n}\langle \bLambda, \vlambda \rangle^2   \right| \nonumber \\
	\leq & \sup\limits_{\|\vlambda\|_{\infty} \leq K}\left| \frac{ \frac{1}{{nd}}\langle \bLambda, \vlambda \rangle^2\left(\|\bTheta\|_2^2 - dq_{\Theta} \right)}{2q_{\Theta}^{-1} +  \frac{2}{\sqrt{nd}}\|\vlambda\|_2^2} \right| +\sup\limits_{\|\vlambda\|_{\infty} \leq K} \left| \frac{\frac{1}{n}q_{\Theta}^2 \langle \bLambda, \vlambda \rangle^2 \times \frac{1}{\sqrt{nd}}\|\vlambda\|_2^2}{2q_{\Theta}^{-1} + \frac{2}{\sqrt{nd}}\|\vlambda\|_2^2} \right|\nonumber \\
	\leq & \frac{nK^4 q_{\Theta}}{2d} \left| \|\bTheta\|_2^2 - d q_{\Theta} \right| + \frac{q_{\Theta}^3n^{3/2}K^6}{2d^{1/2}}, \label{eq:225} \\
	& \sup\limits_{\|\vlambda\|_{\infty} \leq K} \left| \frac{\frac{1}{(nd)^{3/4}}\langle \bLambda, \vlambda \rangle \langle \vlambda ,\bZ\bTheta \rangle}{q_{\Theta}^{-1} + \frac{1}{\sqrt{nd}}\|\vlambda\|_2^2} \right| \leq \frac{n^{3/4}q_{\Theta}K^3}{d^{3/4}}\|\bZ \bTheta\|_2, \label{eq:226} \\
	& \sup\limits_{\|\vlambda\|_{\infty} \leq K}\left| \frac{\left\| \frac{1}{\sqrt[4]{nd}} \bZ^\intercal \vlambda \right\|_2^2}{2q_{\Theta}^{-1} + \frac{2}{\sqrt{nd}}\|\vlambda\|_2^2} - \frac{\left\| \frac{1}{\sqrt[4]{nd}} \bZ^\intercal \vlambda \right\|_2^2}{2q_{\Theta}^{-1}} + \frac{\left\| \frac{1}{\sqrt[4]{nd}} \bZ^\intercal \vlambda \right\|_2^2 \frac{1}{\sqrt{nd}}\|\vlambda\|_2^2}{2q_{\Theta}^{-2}} \right| \leq  \frac{n^2K^6 q_{\Theta}^3}{2d} \times \frac{1}{\sqrt{nd}} \|\bZ\bZ^\intercal\|_{op}, \label{eq:227} \\
	&  \sup\limits_{\|\vlambda\|_{\infty} \leq K} \left| \frac{d}{2} \log \left(1 + \frac{q_{\Theta}}{\sqrt{nd}} \|\vlambda\|_2^2 \right) - \frac{dq_{\Theta}}{2\sqrt{nd}}\|\vlambda\|_2^2 + \frac{q_{\Theta}^2}{4n} \|\vlambda\|_2^4 \right| \leq \frac{d}{2} \times \frac{\left( \sqrt{\frac{n}{d}}K^2 q_{\Theta} \right)^3}{1 - \sqrt{\frac{n}{d}}K^2 q_{\Theta}}. \label{eq:228}
\end{align}
Combining \eqref{eq:225}, \eqref{eq:226}, \eqref{eq:227} and \eqref{eq:228} we get
\begin{align}
	 \left|\Phi_n^{(0)} - \tilde{\Phi}_n \right| \leq &  \frac{1}{n} \E\left[ \frac{nK^4 q_{\Theta}}{2d} \left| \|\bTheta\|_2^2 - d q_{\Theta} \right| + \frac{q_{\Theta}^3n^{3/2}K^6}{2d^{1/2}} + \frac{n^2K^6 q_{\Theta}^3}{2d} \times \frac{1}{\sqrt{nd}} \|\bZ\bZ^\intercal\|_{op} + \frac{d}{2} \times \frac{\left( \sqrt{\frac{n}{d}}K^2 q_{\Theta} \right)^3}{1 - \sqrt{\frac{n}{d}}K^2 q_{\Theta}} + \right. \nonumber \\
	& \left. \frac{q_{\Theta}^2K^4n}{2} \times \left\|\frac{1}{d} \bZ\bZ^\intercal - \id_n\right\|_{op} + \frac{n^{3/4}q_{\Theta}K^3}{d^{3/4}}\|\bZ \bTheta\|_2 \right] \label{eq:229}
\end{align}
By lemma \ref{lemma:concentration-of-sample-covariance}, 
\begin{align}
	\E\left[ \left\| \frac{1}{d} \bZ\bZ^\intercal - \id_n  \right\|_{op} \right] \leq & 100\sqrt{\frac{n}{d}} + \int_{100\sqrt{n/d}}^{\infty} \exp\left( -\frac{dx^2}{3200} \right) \dd x  \leq  100\sqrt{\frac{n}{d}} + \frac{40}{\sqrt{d}}\int_0^{\infty} \exp\left( -\frac{y^2}{2} \right)\dd y. \label{eq:230}
\end{align}
Using \eqref{eq:230}, we conclude from \eqref{eq:229} that $|\Phi_n^{(0)}- \tilde{\Phi}_n  | = o(1) $, thus finishing the proof of this lemma.
\end{proof}
In the $n,d \rightarrow \infty$ limit, $\frac{1}{\sqrt{d}}\left( \bZ\bZ^\intercal - d\id_n \right)$ asymptotically behaves like a GOE$(n)$ matrix, thus inspires us to consider a symmetric matrix model $\bY = \frac{q_{\Theta}}{n} \bLambda \bLambda^\intercal + \bW \in \RR^{n \times n}$, where $\bW \overset{d}{=} \frac{1}{\sqrt{n}}\GOE(n)$. The corresponding free energy density can be expressed as follows:
\begin{align*}
	 \Phi_n^Y = \frac{1}{n} \E\left[ \log \left( \int \exp\left( \frac{q_{\Theta}^2}{2n} \langle \bLambda, \vlambda \rangle^2 + \frac{q_{\Theta}}{2} \vlambda^\intercal\bW\vlambda - \frac{q_{\Theta}^2}{4n}\|\vlambda\|_2^4  \right)\tensorl \right) \right]. 
	%& R_n = \frac{3q_{\Theta}^2}{2n}\sum\limits_{i = 1}^n \Lambda_i^2\lambda_i^2 - \frac{3q_{\Theta}^2}{4n}\sum\limits_{i = 1}^n\lambda_i^4 + \frac{3q_{\Theta}}{2}\sum\limits_{i = 1}^n \lambda_i^2 W_{ii}.
\end{align*}
%\yw{$R_n$ to be dealt with}
The next lemma shows the asymptotic equivalence between $\Phi_n^Y$ and $\tilde{\Phi}_n$:
\begin{lemma}\label{lemma:free-energy-3}
	Under the assumptions stated in Lemma \ref{lemma:free-energy-1}, $\Phi_n^Y - \tilde{\Phi}_n = o(1)$ as $n,d \rightarrow \infty$. 
\end{lemma}

\begin{proof}
	Notice that for any deterministic orthogonal matrix $\bO \in \RR^{n \times n}$, $\bO^\intercal\bW \bO \overset{d}{=} \bW$, $\bO^\intercal (\bZ\bZ^\intercal - \id_n) \bO^\intercal \overset{d}{=} (\bZ\bZ^\intercal - \id_n)$, such matrices then admit the eigen-decomposition 
	\begin{align}
		\frac{1}{\sqrt{nd}}\left( \bZ^\intercal \bZ - d\id_n \right) = \bOmega^\intercal \bS_1 \bOmega, \qquad  \bW = \bOmega^\intercal \bS_2 \bOmega, \label{eq:231}
	\end{align}
	where $\bOmega$ is Haar-distributed on the orthogonal matrix group, $\bS_1$ and $\bS_2$ are diagonal matrices containing acendingly ordered eigenvalues. Furthermore, $\bS_1, \bS_2$ and $\bOmega$ are independent of each other. Note that \eqref{eq:231} naturally provides a way of coupling $\frac{1}{\sqrt{nd}}\left( \bZ^\intercal \bZ - d\id_n \right)$ and $ \bW$. Then we have the upper bound:
	\begin{align*}
		\left|\tilde{\Phi}_n - \Phi_n^Y\right| \leq &  \frac{1}{n} \E\left[ \sup\limits_{\|\vlambda\|_{\infty} \leq K} \left| \frac{q_{\Theta}}{2}\vlambda^\intercal\left( \bW - \frac{1}{\sqrt{nd}}\left(\bZ\bZ^\intercal - d\id_n \right) \right)\vlambda  \right|  \right] \leq \frac{q_{\Theta}K^2}{2} \E\left[ \|\bS_1 - \bS_2\|_{op} \right].
	\end{align*}
	Let $\sigma_i(\bS_j)$ be the $i$-th largest eigenvalue of $\bS_j$, then $\|\bS_1 - \bS_2\|_{op} = \max\limits_{i \in [n]}|\sigma_i(\bS_1) - \sigma_i(\bS_2)|$. Let ESD denote the empirical spectral distribution. By standard results in random matrix theory, ESD$(\bS_1)$ and ESD$(\bS_2)$ both converges almost surely to the semicircle law(\cite{bai1988convergence}). Furthermore, thanks to past literatures \cite{bai1988necessary, paul2012asymptotic, karoui2003largest}, we have $\sigma_1(\bS_1), \sigma_1(\bS_2) \overset{a.s.}{\rightarrow} 2$ and $\sigma_n(\bS_1), \sigma_n(\bS_2) \overset{a.s.}{\rightarrow} -2$, thus $\|\bS_1 - \bS_2\|_{op} \overset{a.s.}{\rightarrow} 0$. By Theorem 1.1 in \cite{bandeira2016sharp}, for any $0 < \epsilon \leq 1 / 2$,
	\begin{align*}
		\E[\|\bW\|_{op}] \leq (1 + \epsilon)\left\{2\sqrt{1 + \frac{1}{n}} + \frac{6}{\sqrt{\log(1 + \epsilon)}} \sqrt{\frac{2\log n}{n}} \right\}.
	\end{align*}
	First let $n \rightarrow \infty$ then let $\epsilon \rightarrow 0^+$ gives $\limsup\limits_{n \rightarrow \infty}\E[\|\bS_2\|_{op}] \leq 2$. Fatou's lemma gives $\liminf\limits_{n \rightarrow \infty} \E[\|\bS_2\|_{op}] \geq 2$, thus $\lim\limits_{n \rightarrow \infty} \E[\|\bS_2\|_{op}] = 2$. Again applying Lemma \ref{lemma:concentration-of-sample-covariance}, for any $\epsilon > 0$, for $M, n$ large enough, 
	\begin{align*}
		\E\left[ \left\| \bS_1 \right\|_{op} \mathbbm{1}\left\{\| \bS_1\|_{op} \geq M \right\} \right] < \epsilon.
	\end{align*}
	Dominated convergence theorem gives $\limsup\limits_{n \rightarrow \infty} \E[\|\bS_1\|_{op} \mathbbm{1}\{\|\bS_1\|_{op} < M\}] \leq 2$, thus $\limsup\limits_{n \rightarrow \infty} \E[\|\bS_1\|_{op} ] \leq 2 + \epsilon$. For the lower bound part, Fatou's lemma gives $\liminf\limits_{n \rightarrow \infty} \E[\|\bS_1\|_{op} ] \geq 2$, thus $\lim\limits_{n \rightarrow \infty}\E[\|\bS_1\|_{op}] = 2$. Finally, Scheffé's lemma gives $\E[\|\bS_1 - \bS_2\|_{op}] \rightarrow 0$, thus completing the proof of this lemma. 	
\end{proof}

Let $\bW'$ be an independent copy of $\bW$. For $h > 0$, define the following Hamiltonians:
\begin{align*}
	H_n(\vlambda, \vtheta, h) =& H_n(\vlambda, \vtheta) + \frac{h}{2n}\langle \bLambda, \vlambda \rangle^2 + \frac{\sqrt{h}}{2}\vlambda^\intercal\bW' \vlambda - \frac{h}{4n}\|\vlambda\|_2^4, \\
	\tilde{H}_n(\vlambda, h) =& \frac{q_{\Theta}^2}{2n}\langle \bLambda, \vlambda \rangle^2 + \frac{q_{\Theta}\left\| \frac{1}{\sqrt[4]{nd}}\bZ^\intercal\vlambda \right\|_2^2}{2} - \frac{dq_{\Theta}}{2\sqrt{nd}}\|\vlambda\|_2^2 - \frac{q_{\Theta}^2}{4n}\|\vlambda\|_2^4 + \frac{h}{2n}\langle \bLambda, \vlambda \rangle^2 + \frac{\sqrt{h}}{2}\vlambda^\intercal\bW' \vlambda - \frac{h}{4n}\|\vlambda\|_2^4,\\
	 H_n^Y(\vlambda, h) = &\frac{q_{\Theta}^2}{2n}\langle \bLambda, \vlambda \rangle^2 + \frac{q_{\Theta}}{2} \vlambda^\intercal\bW\vlambda - \frac{q_{\Theta}^2}{4n}\|\vlambda\|_2^4 + \frac{h}{2n}\langle \bLambda, \vlambda \rangle^2 + \frac{\sqrt{h}}{2}\vlambda^\intercal\bW' \vlambda - \frac{h}{4n}\|\vlambda\|_2^4, \\ 
\end{align*}
as well as the corresponding free energy densities:
\begin{align*}
	\Phi_n(h) = & \frac{1}{n}\E\left[ \log \left( \int \exp\left( H_n(\vlambda, \vtheta, h) \right)\tensorl\tensort \right) \right], \\
	\tilde{\Phi}_n(h) = & \frac{1}{n}\E\left[ \log \left( \int \exp\left( \tilde{H}_n(\vlambda, h) \right)\tensorl \right) \right], \\
	\Phi^Y_n(h) = & \frac{1}{n}\E\left[ \log \left( \int \exp\left( {H}_n^Y(\vlambda, h) \right)\tensorl \right) \right].
\end{align*}
Then we have the following lemma:
\begin{lemma}\label{lemma:free-energy-4}
	Under the assumptions stated in Lemma \ref{lemma:free-energy-1}, we have for all $h \geq 0$,
	\begin{enumerate}
		\item $\Phi_n(h) = \tilde{\Phi}_n(h) + o(1)$,
		\item $\tilde{\Phi}_n(h) = \Phi^Y_n(h) + o(1)$.
		\item $\Phi_n(h), \tilde{\Phi}_n(h)$ and $\Phi^Y_n(h)$ are differentiable, and convex on $(0, \infty)$. 
	\end{enumerate}
\end{lemma}
\begin{proof}
	The proofs of the first two results are almost identical to the proof of Lemma \ref{lemma:free-energy-1}, \ref{lemma:free-energy-2} and \ref{lemma:free-energy-3}. \yw{third result todo}
\end{proof}
We can compute the following derivatives:
\begin{align*}
	\Phi_n'(h) = \frac{1}{4n^2} \E\left[ \left\langle \left(\sum\limits_{i = 1}^n \lambda_i \Lambda_i \right)^2 \right\rangle_h \right],\ \ \tilde{\Phi}_n'(h) = \frac{1}{4n^2} \E\left[ \left\langle \left(\sum\limits_{i = 1}^n \lambda_i \Lambda_i \right)^2 \right\rangle_{h, \sim } \right], \ \ {\Phi_n^{Y }}'(h) = \frac{1}{4n^2} \E\left[ \left\langle \left(\sum\limits_{i = 1}^n \lambda_i \Lambda_i \right)^2 \right\rangle_{h, Y } \right]
\end{align*} 
where $\langle \cdot \rangle_h$, $\langle \cdot \rangle_{h, \sim}$ and $\langle \cdot \rangle_{h, Y}$ are Gibbs measure corresponding to the Hamiltonians $H_n(\vlambda, \vtheta, h)$, $\tilde{H}_n(\vlambda, h)$ and $H_n^Y(\vlambda, h)$, respectively. Following the notations in \cite{lelarge2019fundamental}, let
%\begin{align*}
%	F_n(s) = \frac{1}{n} \E\left[ \log \left( \int \exp\left( \frac{s}{2n}\langle \bLambda, \vlambda \rangle^2 + \frac{\sqrt{s}}{2}\vlambda^\intercal\bW\vlambda - \frac{s}{4n}\|\vlambda\|_2^4 \right)\tensorl \right)  \right].
%\end{align*} 
\begin{align*}
	F_n(s) = \frac{1}{n} \E\left[ \log \left( \int \exp\left( \sum\limits_{i < j }\sqrt{s}\lambda_i\lambda_j W_{ij} + \frac{s}{n}\Lambda_i\Lambda_j \lambda_i\lambda_j - \frac{s}{2n} \lambda_i^2\lambda_j^2 \right)\tensorl \right)  \right],
\end{align*}
Notice that $F_n({h + q_{\Theta}}^2) = \Phi_n^Y(h) + o(1)$. For the sake of completeness, here we reproduce the definition of the following function proposed in \cite{lelarge2019fundamental}:
\begin{align*}
	\cF: (s, q) \in \RR_+^2  \mapsto - \frac{s}{4}q^2 + \E\log \left(\int \exp\left( \sqrt{sq}Z\lambda + sq\lambda \Lambda - \frac{s}{2}q\lambda^2 \right)\dd P_{\Lambda}(\lambda) \right),
\end{align*} 
where $Z \sim \normal(0,1)$. We define
\begin{align*}
	D = \left\{s > 0 \mid \cF(s, \cdot) \mbox{ has only a unique maximizer } q^{\ast}(s) \right\}.
\end{align*}
By Theorem 13 in \cite{lelarge2019fundamental}, $\lim\limits_{n \rightarrow \infty}F_n(s) = \sup\limits_{q \geq 0} \cF(s, q)$. By proposition 17 in \cite{lelarge2019fundamental}, $D$ is equal to $(0, +\infty)$ minus some countable set and is precisely the set of $s > 0$ at which the function $\phi: s \mapsto \sup\limits_{q \geq 0}\cF(s, q)$ is differentiable. Then by Lemma \ref{lemma:convex-derivative}, given $q_{\Theta}$, for almost all $h > 0$, $\lim\limits_{n \rightarrow \infty}\Phi_n'(h) = \lim\limits_{n \rightarrow \infty} {\Phi_n^Y}'(h) = \phi(h + q_{\Theta})$. Let 
\begin{align*}
	\MMSE_n(\bY) = \min\limits_{\hat{M}(\bY)} \frac{1}{n^2} \E\Big[ \Big\| \bLambda\bLambda^\intercal - \hat{M}(\bY) \Big\|_{F}^2 \Big], \qquad \MMSE_n(\bA) = \min\limits_{\hat{M}(\bA)} \frac{1}{n^2} \E\left[ \left\| \bLambda\bLambda^\intercal - \hat{M}(\bA) \right\|_{F}^2 \right].
\end{align*}
Notice that 
\begin{align*}
	{\Phi_n^Y}'(0) = \frac{1}{4n^2} \E\Big[ \Big<\Big( \sum\limits_{i = 1}^n \Lambda_i\lambda_i \Big)^2 \Big>_0 \Big] = \frac{1}{4n^2}\Big( n\E[\Lambda^4] + n(n - 1) \E[\Lambda^2]^2 - n^2\MMSE_n(\bY) \Big)
\end{align*}
Again by Lemma \ref{lemma:convex-derivative}, for almost all $q_{\Theta} > 0$, $\lim\limits_{n \rightarrow \infty}\MMSE_n(\bY) = 4\phi'(q_{\Theta}^2) - \E[\Lambda^2]^2$. Notice that for all $h > 0$, 
\begin{align*}
	\Phi_n'(h) \geq \frac{1}{4n^2} \E\left[ \left<\left( \sum\limits_{i = 1}^n \Lambda_i\lambda_i \right)^2 \right>_0 \right] = \frac{1}{4n^2}\left( n\E[\Lambda^4] + n(n - 1) \E[\Lambda^2]^2 - \MMSE_n(\bA) \right).
\end{align*}
For any $\epsilon > 0$, there exists $h_{\epsilon} > 0$, such that $\phi'(h_{\epsilon} + q_{\Theta}^2) \leq \phi'(q_{\Theta}^2) + \epsilon$(for almost all $q_{\Theta}^2 > 0$ we have $\phi'$ continuous at $q_{\Theta}^2$), and $\phi$ is differentiable at $h_{\epsilon} + q_{\Theta}^2$. Then there exists $n_{\epsilon} \in \NN^+$, such that for all $n \geq n_{\epsilon}$, $|\Phi_n'(h_{\epsilon}) - \phi(h_{\epsilon} + q_{\Theta}^2)| \leq \epsilon$, thus $\MMSE_n(\bA) \geq \lim\limits_{n \rightarrow \infty} \MMSE_n(\bY) - 2\epsilon$. Since $\epsilon$ is arbitrary, we conclude that for almost all $q_{\Theta}^2$, $\liminf\limits_{n \rightarrow \infty} \MMSE_n(\bA) \geq \lim\limits_{n \rightarrow \infty} \MMSE_n(\bY)$.

\subsection{Reduction to bounded support distribution}\label{section:reduction-to-bdd-support}
We show in this section that it suffices to prove Theorem \ref{thm:lower-bound} for $\Lambda$ having bounded support. The proof follows from section 6.2.2 in \cite{lelarge2019fundamental}. For any $\epsilon > 0$, there exists $K_{\epsilon} > 0$, such that if we let $\barLambda = \Lambda \mathbbm{1}\{|\Lambda| \leq K_{\epsilon}\}$, then $\E[(\Lambda - \barLambda)^4] < \epsilon$. Let $\barLambda_i, \bar{\lambda}_i$ be the truncated version of $\Lambda_i$ and $\lambda_i$. Further we let $\bar{\Phi}_n$ and $\bar{\cF}$ be the free energy and function corresponding to truncated random variable $\bar{\Lambda}$. Then we have the following lemma:
\begin{lemma}\label{lemma:bounded-approx-free-energy}
	There exists a constant $C_0 > 0$ that depends only on the law of $\Lambda$ and $\Theta$, such that for all $n,d \in \NN^+$ with $d / n$ large enough, and all $h \in [0,1]$,
	\begin{align*}
		\left| \Phi_n(h) - \bar{\Phi}_n(h)  \right| \leq C_0\sqrt{\epsilon}.
	\end{align*}
\end{lemma}
\begin{proof}
	For the sake of simplicity we prove the result for $h = 0$, and recall that $\Phi_n(0) = \Phi_n$, thus analogously $\bar{\Phi}_n(0) = \bar{\Phi}_n$. Proof for non-zero $h$ values is almost identical. For $t \in [0,1]$, define the following interpolated Hamiltonian:
	\begin{align*}
		H_{n,t}(\vlambda, \vtheta) = & \frac{t}{\sqrt{nd}}\sum\limits_{i \in [n], j \in [d]} \Lambda_i\lambda_i \Theta_j \theta_j + \frac{\sqrt{t}}{\sqrt[4]{nd}} \sum\limits_{i \in [n], j \in [d]} Z_{ij} \lambda_i \theta_j - \frac{t}{2\sqrt{nd}}\sum\limits_{i \in [n], j \in [d]}\lambda_i^2 \theta_j^2 + \\
		& \frac{1 - t}{\sqrt{nd}}\sum\limits_{i \in [n], j \in [d]} \barLambda_i\bar{\lambda}_i \Theta_j \theta_j + \frac{\sqrt{1 - t}}{\sqrt[4]{nd}} \sum\limits_{i \in [n], j \in [d]} Z_{ij}' \bar{\lambda}_i \theta_j - \frac{1 - t}{2\sqrt{nd}}\sum\limits_{i \in [n], j \in [d]}\bar{\lambda}_i^2 \theta_j^2,
	\end{align*}
	where $Z_{ij}'$ being an independent copy of $Z_{ij}$. Notice that this is the Hamiltonian for observations $\bA_1 = \frac{\sqrt{t}}{\sqrt[4]{nd}} \bLambda \bTheta^\intercal + \bZ$ and $\bA_2 = \frac{\sqrt{1 - t}}{\sqrt[4]{nd}} \bar{\bLambda} \bTheta^\intercal + \bZ' $. Let
	\begin{align*}
		\Phi_{n,t} = \frac{1}{n} \E\left[ \log \left( \int \exp\left( H_{n,t}(\vlambda, \vtheta)\right)\tensorl\tensort \right) \right].
	\end{align*}
	Notice that $\Phi_{n,0} = \bar{\Phi}_n$ and $\Phi_{n,1} = {\Phi}_n$. Let $\langle \cdot \rangle_{n,t}$ be the Gibbs measure associated with Hamiltonian $H_{n,t}$. For $0 < t < 1$, by Gaussian integration by parts and Nishimori property, 
	\begin{align*}
		\frac{\dd}{\dd t}\Phi_{n,t} =&  \frac{1}{2n\sqrt{nd}} \sum\limits_{i \in [n], j \in [d]} \E\left[ \langle (\Lambda_i \lambda_i - \barLambda_i \bar{\lambda}_i) \Theta_j \theta_j \rangle_{n,t} \right] \\
		=& \frac{1}{2\sqrt{nd}} \E\left[ \left\langle(\Lambda_1 \lambda_1 - \barLambda_1 \bar{\lambda}_1) \langle \bTheta, \vtheta \rangle \right\rangle_{n,t} \right] \\
		\leq & \frac{1}{2\sqrt{nd}} \E\left[\left\langle(\Lambda_1 \lambda_1 - \barLambda_1 \bar{\lambda}_1)^2 \right\rangle_{n,t}^{1/2}\left\langle  \langle \bTheta, \vtheta \rangle^2 \right\rangle_{n,t}^{1/2}\right] \\
		\leq & \frac{1}{2\sqrt{nd}} \E\left[\left\langle(\Lambda_1 \lambda_1 - \barLambda_1 \bar{\lambda}_1)^2 \right\rangle_{n,t} \right]^{1/2}\E\left[\left\langle\langle \bTheta, \vtheta \rangle^2 \right\rangle_{n,t} \right]^{1/2}.
	\end{align*}
	Denote $\langle \cdot \rangle_{n,t,\ast}$ the Gibbs measure given observation $(\bA_1, \bA_2, \bLambda, \bar{\bLambda})$.  Notice that
	\begin{align}
		\E\left[\left\langle\langle \bTheta, \vtheta \rangle^2 \right\rangle_{n,t} \right] =& d\E\left[\left\langle \Theta_1^2\theta_1^2  \right\rangle_{n,t}\right] + d(d - 1)\E\left[\left\langle \Theta_1\Theta_2\theta_1\theta_2  \right\rangle_{n,t}\right] \nonumber \\
		\leq & d\E[\Theta_1^4] + d(d - 1) \E\left[\left\langle \Theta_1\Theta_2\theta_1\theta_2  \right\rangle_{n,t, \ast}\right]. \label{eq:232}
	\end{align}
	Recall that $F_{\Theta}(\delta) = \sqrt{\frac{d}{n}} \E\left[ \E\left[ \Theta \mid \sqrt[4]{nd^{-1}}\delta \Theta + G \right]^2 \right]$, then we have
	\begin{align}
		\E\left[\left\langle \Theta_1\Theta_2\theta_1\theta_2  \right\rangle_{n,t, \ast}\right] \leq \frac{n}{d}\E\left[ F_{\Theta}\left( \sqrt{({t\|\bLambda\|_2^2 + (1 - t)\|\barLambda\|_2^2})/{n}} \right)^2 \right].  \label{eq:233}
	\end{align}
	Following \eqref{eq:188}, notice that $G \sim \normal(0,1)$, and recall that we have defined $r_n = n^{-1/4}d^{1/4}$ in Section \ref{sec:weak-signal}, then we have
	\begin{align*}
		\left|\frac{\dd}{\dd\delta} \E\left[ \Theta \mid r_n^{-1} \delta \Theta + G \right] \right| \leq & r_n^{-1} \times \left\{ 2r_n^{-1} \delta |\Theta| \Var\left[ \Theta \mid r_n^{-1} \delta \Theta + G  \right] + |G|\Var\left[ \Theta \mid r_n^{-1} \delta \Theta + G  \right]   \right. \\
		& \left. + r_n^{-1} \delta \E[|\Theta|^3 \mid r_n^{-1} \delta \Theta + G] + r_n^{-1} \delta \E[\Theta^2 \mid r_n^{-1} \delta \Theta + G]\E[|\Theta|\mid r_n^{-1} \delta \Theta + G] \right\}. 
	\end{align*}
	Therefore, we further have
	\begin{align*}
		F_{\Theta}(\delta) =& \sqrt{\frac{d}{n}} \E\left[ \E[\Theta \mid r_n^{-1} \delta \Theta + G]^2 \right] \\
		\leq & \sqrt{\frac{d}{n}} \E\left[ \left( \int_0^{\delta} \left|\frac{\dd}{\dd\delta} \E\left[ \Theta \mid r_n^{-1} \delta \Theta + G \right] \right| \dd \delta \right)^2\right] \\
		\leq & \sqrt{\frac{d}{n}} \E\left[ \delta \int_0^{\delta} \left|\frac{\dd}{\dd\delta} \E\left[ \Theta \mid r_n^{-1} \delta \Theta + G \right] \right|^2 \dd \delta\right] \\
		\leq & 4\delta \E\left[ \int_0^{\delta} 4r_n^{-2} \delta^2 \Theta^2 \Var\left[ \Theta \mid r_n^{-1} \delta \Theta + G  \right]^2 + G^2 \Var\left[ \Theta \mid r_n^{-1} \delta \Theta + G  \right]^2 \right. \\
		& \left. + r_n^{-2} \delta^2\E[|\Theta|^3 \mid r_n^{-1} \delta \Theta + G]^2 + r_n^{-2} \delta^2 \E[\Theta^2 \mid r_n^{-1} \delta \Theta + G]^2\E[|\Theta|\mid r_n^{-1} \delta \Theta + G]^2 \dd\delta  \right] \lesssim  C(\delta^4 + 1),
	\end{align*}
	where $C$ is a numerical constant that depends only on the law of $\Theta$.

	Let $S = \left\{ \|\bLambda\|_2^2 \leq n\E[\Lambda^2] + n\|\Lambda^2\|_{\Psi_1} \right\}$, where $\|\cdot\|_{\Psi_1}$ is the sub-exponential norm of $\Lambda^2$. Then there exists numerical constant $c > 0$, such that for all $s \geq 1$,
	\begin{align*}
		\P\left( \|\bLambda\|_2^2 \geq n\E[\Lambda^2] + sn\|\Lambda^2\|_{\Psi_1} \right) \leq 2\exp\left( -cns \right). 
	\end{align*}
	Then we have
	\begin{align}
		& \frac{n}{d}\E\left[ F_{\Theta}\left( \sqrt{({t\|\bLambda\|_2^2 + (1 - t)\|\barLambda\|_2^2})/{n}} \right)^2 \right] \nonumber \\
		=& \frac{n}{d}\E\left[ F_{\Theta}\left( \sqrt{({t\|\bLambda\|_2^2 + (1 - t)\|\barLambda\|_2^2})/{n}} \right)^2 \mathbbm{1}_S \right] + \frac{n}{d}\E\left[ F_{\Theta}\left( \sqrt{({t\|\bLambda\|_2^2 + (1 - t)\|\barLambda\|_2^2})/{n}} \right)^2 \mathbbm{1}_{S^c} \right]\nonumber \\
		\leq & \frac{4C^2n}{d} + \frac{2C^2n}{d}\left( \E[\Lambda^2] + \|\Lambda^2\|_{\Psi_1} \right)^4 + \frac{2nC^2}{d} \E\left[ \left(\|\bLambda\|_2^2 / n \right)^4\mathbbm{1}_{S^c}  \right]\nonumber \\
		\leq & \frac{4C^2n}{d} + \frac{2C^2n}{d}\left( \E[\Lambda^2] + \|\Lambda^2\|_{\Psi_1} \right)^4 + \frac{2nC^2}{d} \int_1^{\infty} 4\P\left( \frac{1}{n}\|\bLambda\|_2^2 \geq \E[\Lambda^2] + s\|\Lambda^2\|_{\Psi_1} \right)\left(\E[\Lambda^2] + s\|\Lambda^2\|_{\Psi_1} \right)^3\|\Lambda^2\|_{\Psi_1} \dd s\nonumber \\
		\leq & \frac{4C^2n}{d} + \frac{2C^2n}{d}\left( \E[\Lambda^2] + \|\Lambda^2\|_{\Psi_1} \right)^4 + \frac{2nC^2}{d}\int_1^{\infty}8\exp\left( -cns \right)\left(\E[\Lambda^2] + s\|\Lambda^2\|_{\Psi_1} \right)^3\|\Lambda^2\|_{\Psi_1} \dd s \leq \frac{C_1n}{d}, \label{eq:234}
	\end{align}
	where $C_1$ is dependent only on the law of $\Lambda, \Theta$, and especially, independent of $n$ and $d$. Furthermore, we have
	\begin{align}
		\E\left[\left\langle(\Lambda_1 \lambda_1 - \barLambda_1 \bar{\lambda}_1)^2 \right\rangle_{n,t} \right] \leq & 2\E\left[ \Lambda_1^2 \langle (\lambda_1 - \bar{\lambda}_1)^2 \rangle_{n,t} \right] + 2\E\left[(\Lambda_1 - \bar{\Lambda}_1)^2\langle  \bar{\lambda}_1^2 \rangle_{n,t}   \right] \nonumber \\
		\leq & 2\E\left[ \Lambda_1^4  \right]^{1/2} \E\left[ \langle (\lambda_1 - \bar{\lambda}_1)^2  \rangle_{n,t}^2  \right]^{1/2} + 2\E\left[(\Lambda_1 - \barLambda_1)^4 \right]^{1/2} \E\left[ \langle \bar{\lambda}_1^2 \rangle^2 \right]^{1/2} \nonumber \\
		\leq & 2\E\left[ \Lambda_1^4  \right]^{1/2}\E\left[ (\Lambda_1 - \barLambda_1)^4  \right]^{1/2} + 2\E\left[(\Lambda_1 - \barLambda_1)^4 \right]^{1/2}\E\left[ \bar{\Lambda}_1^4 \right] \leq C_2 \sqrt{\epsilon},\label{eq:235}
	\end{align}
	where $C_1$ is dependent only on the law of $\Lambda$, and especially, independent of $n$ and $d$. Combining \eqref{eq:232}, \eqref{eq:233}, \eqref{eq:234} and \eqref{eq:235}, we have
	\begin{align*}
		\left|\frac{\dd}{\dd t}\Phi_{n,t}\right| \leq C_0 \sqrt{\epsilon},
	\end{align*}
	where $C_0$ is a constant that depends only on the law of $\Lambda, \Theta$ and is independent of $n,d$, thus finishing the proof of Lemma \ref{lemma:bounded-approx-free-energy}.  	
	
\end{proof}

For the sake of completeness, here we reproduce Lemma 46 and Theorem 41 from \cite{lelarge2019fundamental}.
\begin{lemma}\label{lemma:from-LM19}
\begin{enumerate}
	\item There exists a constant $K' > 0$ that depends only on the law of $\Lambda$, such that
	\begin{align*}
		\left| \sup\limits_{q > 0} \cF(s, q) - \sup\limits_{q > 0} \bar{\cF}(s,q) \right| \leq sK'\epsilon.
	\end{align*}
	\item $\lim\limits_{n \rightarrow \infty} F_n(s) = \sup\limits_{q > 0} \cF(s,q)$.
\end{enumerate}
\end{lemma}
Combining Lemma \ref{lemma:bounded-approx-free-energy} and \ref{lemma:from-LM19}, we conclude that Lemma \ref{lemma:free-energy-4} holds for any $\Lambda$ having sub-gaussian distributions, thus relaxes the conditions of Theorem \ref{thm:lower-bound}.
